# Supplementary material for: An Optimization algorithm for nonsmooth nonconvex problems with upper-C^2 objective
Source: arXiv:2204.09631 source file (2022-04-20)
Supplement: Supplementary file 1 [file Appendix.tex]

%%%%%%%%%%%%%%%%%%%%%%%%%%%%%%%%% APPENDIX %%%%%%%%%%%%%%%%%%%%%%%%%%%%%%%%%%%%%
\setcounter{section}{1}

\addcontentsline{toc}{section}{Appendix A: Slicing algorithm} 
%-------------------------------------------------------------------------------
\section*{Appendix A: Continuity of the second-stage solution function}\label{sec:cont}
\par\noindent
This appendix details the one-sided slicing algorithm in two dimensions. 
We first consider continuity of $r_{\mu}(x)$ using Proposition 4.4 from~\cite{shapiro2000}. The related notations
are denotes as follows.
The set $S(x)\in Y$ is the optimal solutions at $x$.
We denote by $\Phi(x) \subset \Rbb^m$ the feasible set of $y$ in the recourse subproblem.
From the constraints in~\eqref{eqn:opt-rc-mu-al}, an important observation is that $\Phi(x)=\Phi$, for all x, \textit{i.e.} the 
feasible set for $y$ is independent of $x$ due to smoothing.
 To simplify 
the notations instead of applying compact set theories on the extended real vector space, it is reasonable to assume the following.
\begin{assumption}\label{assp:compact-set}
 The optimization variables $x$ and $y$ are bounded. The feasibility sets for $x$ and $y$, denoted as $X\in \Rbb^n$ and $Y\in\Rbb^m$, respectively, are compact.
\end{assumption}
We establish in Lemma~\ref{lem:continuity} that under the given assumption, 
the optimization problem in~\eqref{eqn:opt-rc-mu-al} meets the conditions in Proposition 4.4 in~\cite{shapiro2000}, which 
directly establishes the continuity of $r_{\mu}(x)$.

\begin{lemma}\label{lem:continuity}
The optimization problem~\eqref{eqn:opt-rc-mu-al} satisfies the conditions in Proposition 4.4 in~\cite{shapiro2000} at a given x,
which are (1) the function $f(x,y)$ is continuous
on $X \times Y$, (2) the multifunction $\Phi(\cdot)$ is closed, (3) there exists $\alpha\in \Rbb$ and a compact
set $C\subset Y$ such that for every $x'$ in a neighborhood of $x$, the level set
\begin{equation} \label{eqn:inf-compactness}
 \centering
  \begin{aligned}
	  \text{lev}_{\alpha}f(x',):=\{y \in \Phi(x): f(x',y)\leq \alpha \}
  \end{aligned}
\end{equation}
is nonempty and contained in C, (4)
for any neighborhood $V_y$ of the set $S(\bar{x})$,$\bar{x}\in X$, there exists a neighborhood $V_x$ of $\bar{x}$ such that
$V_y\cap \Phi(x)\neq \emptyset$ for all $x \in V_x$.
\end{lemma}
\begin{proof}
The objectives and constraints in the recourse subproblem are twice continuously differentiable, as mentioned 
	when introducing~\eqref{eqn:2ndstage},
	which guarantees (1) for the entire feasible set $\Phi(x)$. Assumption~\ref{assp:compact-set}, consistent with 
the constraints and bounds on $y$, ensures a closed feasible set and thus (2) is met. 
Since $f(x',y)$ is continuously differentiable on $X \times Y$, it is also bounded.
Denoting a neighborhood of $x$ as $V_x$, 
the obvious choice of $\alpha$ to make the level set $\text{lev}_{\alpha}f(x',),  \forall x' \in V_x$ nonempty is to let it be the maximum value of $f(x',)$ on $C$. Therefore, an $\alpha$ exists such that $f(x',y)\leq \alpha, \forall x' \in V_x,y\in \Phi(x')$.
	Given the compact set $Y\subset \Rbb^m$, 
a compact subset $C\subset Y$ can be found such that the level set $\text{lev}_{\alpha}f(x',)$ is contained in $C$. 
Thus, (3) is satisfied.
To see (4),
	let $\bar{y} \in S(\bar{x})$ and $V_{y}$ be a neighborhood of $\bar{y}$. Since $\Phi(x)$ is independent of $x$
and compact, it is clear $V_y\cap \Phi(x)\neq \emptyset$.
\end{proof}
We can then prove Lemma~\ref{lemma:continuity}.

\begin{proof}
Applying Proposition 4.4 in~\cite{shapiro2000} and Lemma~\ref{lem:continuity} directly,  $r_{\mu}(x)$ is continuous for any $x\in X$ and the multifunction $x\to S(x)$ is upper semicontinuous at $x$.
\end{proof}
